# Supplementary material for: Jarvis: Large-scale Server Monitoring with Adaptive Near-data Processing
Source: arXiv:2202.06021 source file (2023-01-29)
Supplement: Supplementary file 1 [file appendices.tex]

\begin{appendices}
\section{Compute cost of optimal query partitioning}
\label{sec:appendix-optimal-partitioning}
Consider the hierarchical architecture of resource nodes in Figure~\ref{fig:arch-monitoring-scale} where each node in the tree topology can communicate with its parent node. A query with $M$ operators are to be executed on monitoring stream being generated on \client{}s. Each \client{} has a query instance which can be represented as a computational pipeline of operators as vertices and edges denoting dataflow dependencies. On the \server{} side, a fixed number of compute nodes are provisioned for processing the query on data from all \client{}s. Each \client{} needs to identify operators which need to be executed locally vs. those that require remote execution on parent node. Due to dataflow dependencies, we can $partition$ the query graph at $M+1$ possible locations in the graph i.e. a partition splits the operators into two sets. Operators before the partition point are executed on \client{} and those after the partition are executed remotely. As an example, for a \client{} $i$ with $M=4$ operators, $p_i \epsilon [0,M]$ represents the operator where partition occurs. So $p_i=3$ means first 3 operators execute on \client{} and the last operator executes remotely.  

Compute resources on \server{} are used to process operators sent for remote execution after partitioning. Data transport also incurs a network overhead cost. Our goal is to parallelize query processing between compute resources on \client{} and \server{} nodes, while minimizing the utilization of finite compute and network resources on \server{}. As we increase the number of \client{}s, processing load increases on the system. And the processing load from different \client{}s can result in network/compute bottleneck on \server{}, hurting query processing time. Thus, we cannot independently partition operators for each \client{}, instead joint partitioning decision needs to be made across \client{}s. When the remote resources are saturated, it is more beneficial for the \client{} to execute operators locally to avoid long processing time. 

Let \textbf{p} denote the partitioning profile for a query, where $p_i$ denotes query partition point for $i^{th}$ \client{}. We now define the following query partitioning problem as follows:
\begin{align*}
    & \displaystyle \min_{\textbf{p}} \sum_{i=1}^{N_{d}}\sum_{j=1}^{M} c_j x_{ij}\\
    subject\ to,&\\
    & T_{local}(i,p_{i}) <= T_{remote}(i,p_{i})\ \forall p_{i}>0, i\epsilon[1,N_{d}]
\end{align*}
Here $x_{ij}$ indicates if partition point of $i^{th}$ \client{} is $j$, $c_j$ is the processing cost on \server{} due to partitioning the query on \client{} at $j^{th}$ operator, $T_{local}(i,p_{i})$ computes the local computation time cost for operators 1 to $p_{i}$ on the $i^{th}$ \client{} node and $T_{remote}(i,p_{i})$ denotes the network transmission time cost of intermediate data from $p_{i}^{th}$ operator to its parent node along with computation time cost of executing operators $p_{i}+1$ till $M$ on the parent node. We want to incentivize executing operators on \client{} so the partitioning costs are ordered as $c_1>c_2>,...>c_M$.

Unfortunately, solving the partitioning problem is extremely challenging.  
\begin{theorem}
Query partitioning problem to distribute query operators across \client{} and \server{} nodes, with the objective of maximizing the resource utilization of \client{} nodes without degrading query processing time, is NP-hard. 
\end{theorem}
\begin{proof}
% Following is the definition for NP-hard problem for maximum cardinality bin packing~\cite{max-cardinality-bin-packing,central-placement-hard}: we are given $N$ items with sizes $p_i$ for $i \epsilon [1,N]$, and $M$ bins of capacity $C$, and the objective is to assign maximum number of items to the fixed number of bins without violating capacity constraint. It can be stated as below:

We introduce the generalized assignment problem (GAP)~\cite{gap} which finds a minimum cost assignment of $n$ items to $m$ bins such that each item is assigned to precisely one bin subject to capacity restrictions on the bin. Following is the definition:
\begin{align*}
    &min\ \sum_{i=1}^{m}\sum_{j=1}^{n} c_{ij} x_{ij}\\
    subject\ to,&\\
    &\sum_{i=1}^{m} x_{ij} = 1, j\epsilon\{1,...,n\},\\
    &\sum_{j=1}^{n} w_{ij} x_{ij} \le b_i, i\epsilon\{1,...,m\},\\
    &x_{ij} \epsilon {0,1}, i\epsilon\{1,...,m\}, j\epsilon\{1,...,n\}\\
\end{align*}
where $c_{ij}$ is the cost associated with assigning item $j$ to bin $i$, $w_{ij}$ the claim on the capacity of bin $i$ by item $j$ if it is assigned to bin $i$, $b_i$ the capacity of bin $i$ and $x_{ij}$ a 0-1 variable indicating whether item $j$ is assigned to bin $i$ ($x_{ij}=1$) or not ($x_{ij}=0$). This problem is known to be NP-hard~\cite{gap}.

% \begin{align*}
%     &min\ \sum_{i=1}^{N}\sum_{j=1}^{M} x_{ij}\\
%     subject\ to,&\\
%     &\sum_{i=1}^{N} w_{i}x_{ij} \le C\ \forall\ j\epsilon[1,M],\\
%     &\sum_{j=1}^{M} x_{ij} \le 1\ \forall\ i\epsilon[1,N],\\
%     &x_{ij} \epsilon {0,1}\ \forall\ i\epsilon[1,N], j\epsilon[1,M]\\
% \end{align*}
% This problem is known to be NP-hard~\cite{max-cardinality-bin-packing}. 
A \client{} $n$ can execute operators remotely with partitioning $p_{n}$ while improving query processing time, if and only if resource usage on \server{} due to remaining \client{}s is below a threshold data rate $D_{n}$ i.e. $\displaystyle \sum_{i\epsilon [1,N]\setminus\{n\}:p_i=p_n} d_i(p_i) < D_{n}$. Here, $d_i(p_i)$ is a function that provides rate of data leaving \client{} $i$ given the partitioning $p_i$ and $D_n$ is the threshold data rate for all the remaining nodes with partitioning $p_n$ so that \client{} $n$ with $p_n$ has enough resources to execute operators remotely. We use the data rate as a measure for the network and compute overhead on the \server{}. Based on this, we transform generalized assignment problem to a special case of our problem of configuring minimum number of \client{}s to execute operators remotely. We can regard the items and bins in GAP as the \client{} nodes and possible partitioning values i.e. possible values in \textbf{p} in our problem, respectively. Then the weight of an item $n$ assigned to bin $m$ is $w_{mn}=d_n(p_n)$ where $m=p_n$, capacity constraint of each bin $b_m=D_{n} + d_n(p_n)$ and cost of each assignment $c_{mn}=c_{p_n}$. Here, $c_{n1}>...>c_{nM}$. By this, we can ensure that as long as \client{} $n$ on its assigned partition $p_n$ is able to improve processing time compared to executing the query locally, total size of items assigned to bin $p_n$ will not violate capacity constraint $b_{p_n}$. This is because $\displaystyle \sum_{i\epsilon [1,N]\setminus\{n\}:p_i=p_n} d_i(p_i) < D_{n}$ which implies $\sum_{j=1}^{n} w_{nj} x_{nj}=\displaystyle \sum_{i\epsilon [1,N]\setminus\{n\}:p_i=p_n} d_i(p_i) + d_n(p_n) < b_{p_n}$.

Therefore, if we have an algorithm that can minimize the number of operators sent to the \server{} without sacrificing processing time, then we can also obtain optimal solution to GAP. Since GAP is NP-hard, our problem is also NP-hard. 
\end{proof}

The key idea of the proof is that GAP can be reduced to a special case of our query partitioning problem. We note that previous works have also established the hardness of optimal query partitioning in other related domains~\cite{central-placement-hard,placement-scheduling-in-mec-arch}. In this paper, we investigate a greedy heuristic approach which is embarrassingly parallel, for making partitioning decisions. We enable the potential latency overhead resulting from our greedy solution to be bound by an upper limit, by configuring the processing duration or epoch for making partitioning decisions. Our approach is implemented in a fully decentralized manner to ensure high scalability of our partitioning system.

\end{appendices}
